# Supplementary material for: Elements
Source: arXiv:1510.00369 source file (2015-09-30)
Supplement: Supplementary file 1 [file Appendix13i.tex]

\vskip1cm

\centerline{
\sambigrm  Appendix}

\vskip1em

\centerline{
Example: Expanded proof of Balrog 13i}

\vskip 2em
Nelson's {\it qea} proof system consists
of a Perl script
which reads the TeX source code, and checks the proof correctness
and generates an expanded version of the proof.
The {\it Balrog} and {\it Elements} documents
contained active hyperlinks, in a blue font,
to these expanded proofs.

As an example, the expanded version
of the proof of {\it 13i.}\ in {\it Balrog} as
generated by {\it qea} is shown below.

\vskip 4em

\hrule

\vskip4em

\def\red#1{\hbox{\textRed{$#1$}\textBlack}}

\parindent=0pt

\raggedright

	\overfullrule=0pt \parskip=\medskipamount
	\centerline{\bf Proof of Theorem 13i}

\bigskip

	\quad The theorem to be proved is

 $  x + 0 = 0 + x \imp \'S' x + 0 = 0 + \'S' x  $

	\quad Suppose the theorem does not hold. Then, with the variables held fixed,

 $(\ro H)\quad [ [ ( x + 0 ) = ( 0 + x ) ] \and [ \neg ( ( \'S' x ) + 0 ) = ( 0 + ( \'S' x ) ) ] ]  $

	\bigskip

 \centerline{\bf Special cases of the hypothesis and previous results:}\bigskip

\leavevmode\phantom00:\quad$0 + x = x + 0 $\qquad from\quad $ /\ro H : x $

\leavevmode\phantom01:\quad$\neg ( \'S' x ) + 0 = 0 + ( \'S' x ) $\qquad from\quad $ /\ro H : x $

\leavevmode\phantom02:\quad$( \'S' x ) + 0 = \'S' x  $\qquad from\quad $ \yy\pdfKlink{12}{http://math.princeton.edu/~nelson/ref/12.pdf}\zz  ; \'S' x  $

\leavevmode\phantom03:\quad$\'S' ( 0 + x ) = 0 + ( \'S' x ) $\qquad from\quad $ \yy\pdfKlink{12}{http://math.princeton.edu/~nelson/ref/12.pdf}\zz  ; 0 ; x $

\leavevmode\phantom04:\quad$x + 0 = x $\qquad from\quad $ \yy\pdfKlink{12}{http://math.princeton.edu/~nelson/ref/12.pdf}\zz  ; x $

\bigskip

\centerline{\bf Equality substitutions:}

\bigskip

\leavevmode\phantom05:\quad$\neg 0 + x = x + 0 \or \neg \'S' ( \red{0 + x} ) = 0 + ( \'S' x ) \or \'S' ( \red{x + 0} ) = 0 + ( \'S' x ) $\medskip

\leavevmode\phantom06:\quad$\neg ( \'S' x ) + 0 = \'S' x  \or \red{( \'S' x ) + 0} = 0 + ( \'S' x ) \or\neg \red{\'S' x} = 0 + ( \'S' x ) $\medskip

\leavevmode\phantom07:\quad$\neg x + 0 = x \or \neg \'S' ( \red{x + 0} ) = 0 + ( \'S' x ) \or \'S' ( \red{x} ) = 0 + ( \'S' x ) $\medskip

\bigskip

\centerline{\bf Inferences:}\openup1\jot

\bigskip

\leavevmode\phantom08:\quad$\neg \'S' ( 0 + x ) = 0 + ( \'S' x ) \or \'S' ( x + 0 ) = 0 + ( \'S' x ) $\qquad by \hfill\break\phantom.\qquad0: $\red{0 + x = x + 0 }$\quad \hfill\break\phantom.\qquad5: $\red{\neg 0 + x = x + 0 }\or \neg \'S' ( 0 + x ) = 0 + ( \'S' x ) \or \'S' ( x + 0 ) = 0 + ( \'S' x ) $

\leavevmode\phantom09:\quad$\neg ( \'S' x ) + 0 = \'S' x  \or \neg 0 + ( \'S' x ) = \'S' x  $\qquad by \hfill\break\phantom.\qquad1: $\red{\neg ( \'S' x ) + 0 = 0 + ( \'S' x ) }$\quad \hfill\break\phantom.\qquad6: $\neg ( \'S' x ) + 0 = \'S' x  \or \red{( \'S' x ) + 0 = 0 + ( \'S' x ) }\or \neg 0 + ( \'S' x ) = \'S' x  $

10:\quad$\neg 0 + ( \'S' x ) = \'S' x  $\qquad by \hfill\break\phantom.\qquad2: $\red{( \'S' x ) + 0 = \'S' x  }$\quad \hfill\break\phantom.\qquad9: $\red{\neg ( \'S' x ) + 0 = \'S' x  }\or \neg 0 + ( \'S' x ) = \'S' x  $

11:\quad$\'S' ( x + 0 ) = 0 + ( \'S' x ) $\qquad by \hfill\break\phantom.\qquad3: $\red{\'S' ( 0 + x ) = 0 + ( \'S' x ) }$\quad \hfill\break\phantom.\qquad8: $\red{\neg \'S' ( 0 + x ) = 0 + ( \'S' x ) }\or \'S' ( x + 0 ) = 0 + ( \'S' x ) $

12:\quad$\neg \'S' ( x + 0 ) = 0 + ( \'S' x ) \or 0 + ( \'S' x ) = \'S' x  $\qquad by \hfill\break\phantom.\qquad4: $\red{x + 0 = x }$\quad \hfill\break\phantom.\qquad7: $\red{\neg x + 0 = x }\or \neg \'S' ( x + 0 ) = 0 + ( \'S' x ) \or 0 + ( \'S' x ) = \'S' x  $

13:\quad$\neg \'S' ( x + 0 ) = 0 + ( \'S' x ) $\qquad by \hfill\break\phantom.\qquad10: $\red{\neg 0 + ( \'S' x ) = \'S' x  }$\quad \hfill\break\phantom.\qquad12: $\neg \'S' ( x + 0 ) = 0 + ( \'S' x ) \or \red{0 + ( \'S' x ) = \'S' x  }$

14:\quad$QEA$\qquad by \hfill\break\phantom.\qquad11: $\red{\'S' ( x + 0 ) = 0 + ( \'S' x ) }$\quad \hfill\break\phantom.\qquad13: $\red{\neg \'S' ( x + 0 ) = 0 + ( \'S' x ) }$

\bye
